# Supplementary material for: Studying How to Efficiently and Effectively Guide Models with Explanations
Source: arXiv:2303.11932 source file (2024-07-21)
Supplement: Supplementary file 1 [file A-qualitative-pareto.tex]

\subsection{Visualizing the Pareto front}
\label{supp:sec:main:qualitative:pareto}
To better understand the differences between models across the Pareto fronts (cf.\ \cref{fig:epg_voc,fig:epg_coco}), in \cref{fig:supp:pareto_front_quali} we show the attribution maps of all \bcos models that are optimized via the \epgloss loss at the input layer, which lie on the Pareto front for the \cocos dataset for multiple examples (rows). In the columns, we plot the attributions from the models on the Pareto front, ordered in decreasing order of \epg score (\ie in the same left-to-right order as shown in \cref{fig:supp:pareto_front_quali:b}). We find a clear correspondence between the \epg score and how much the attributions visually appear to `focus' on the object bounding box.
\begin{figure}[hb]
    \centering
    \textbf{Pareto-front visualization (\cocos).}\\\vspace{.25cm}
    \begin{subfigure}[c]{.76\textwidth}
    \includegraphics[width=\textwidth]{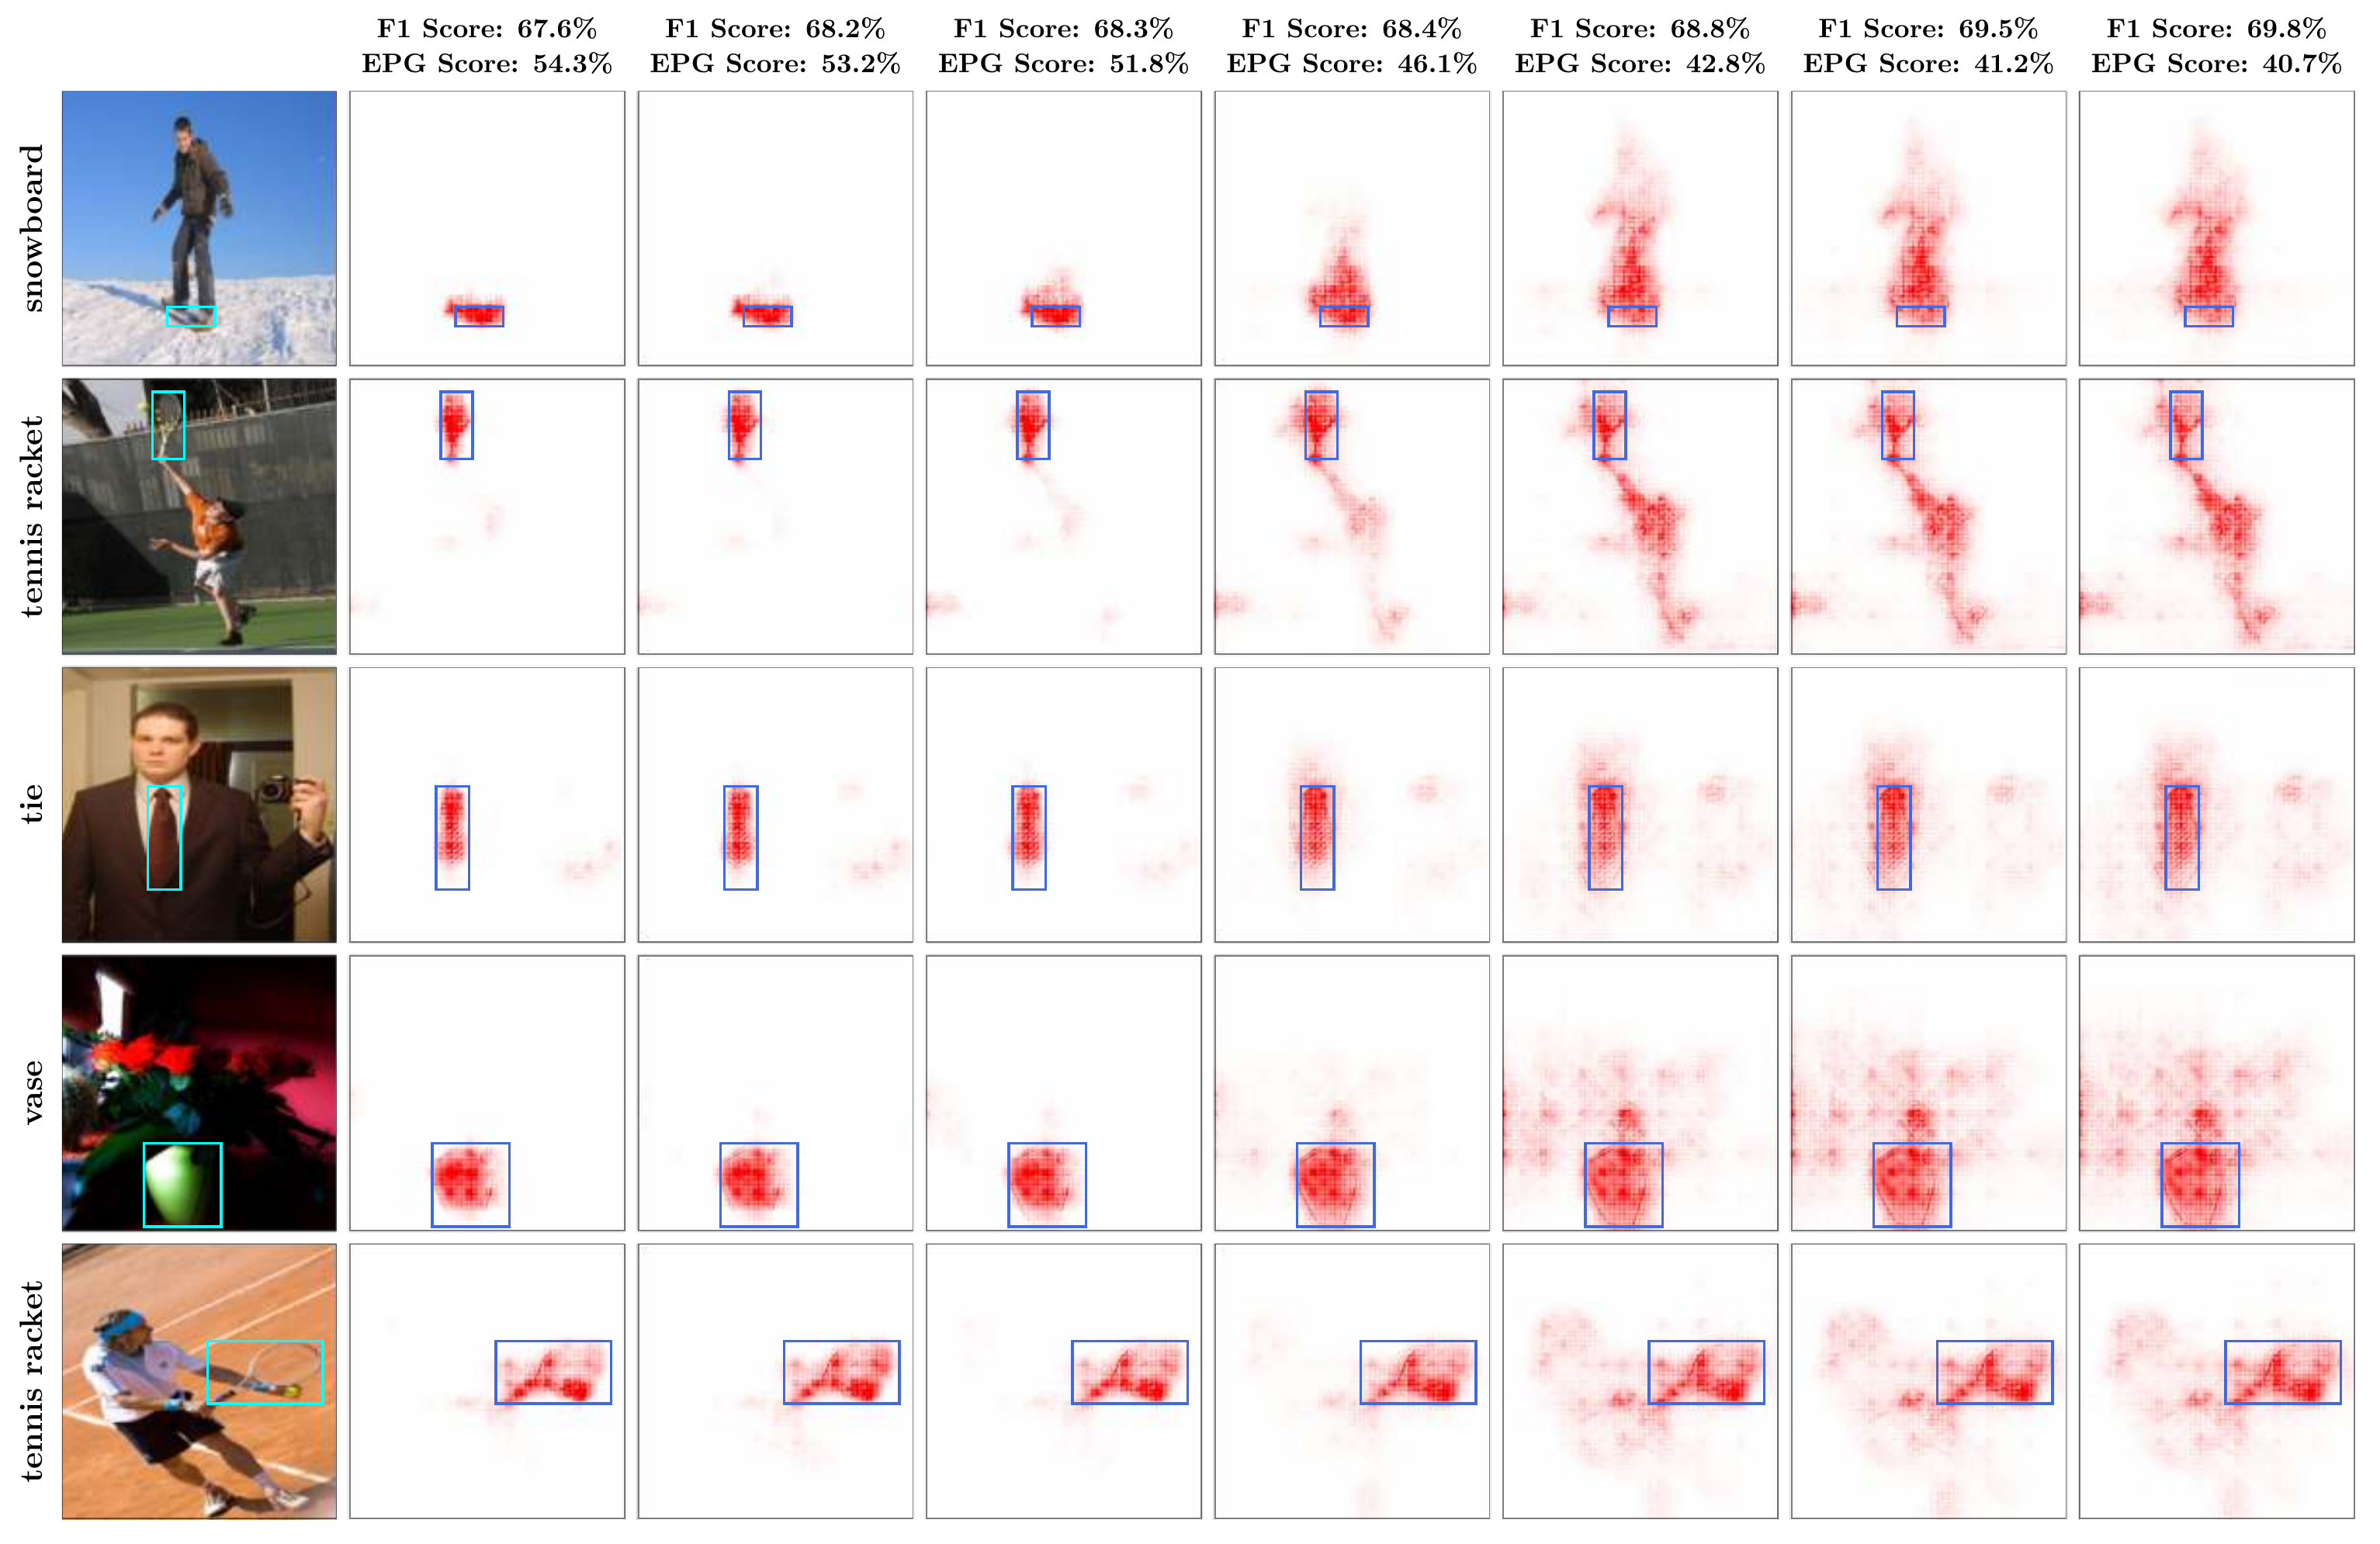}
    \caption{\textbf{Qualitative Examples from across the Pareto front.}}
    \label{fig:supp:pareto_front_quali:a}
    \end{subfigure}\hfill
    \begin{subfigure}[c]{.2275\textwidth}
    \includegraphics[width=\textwidth]{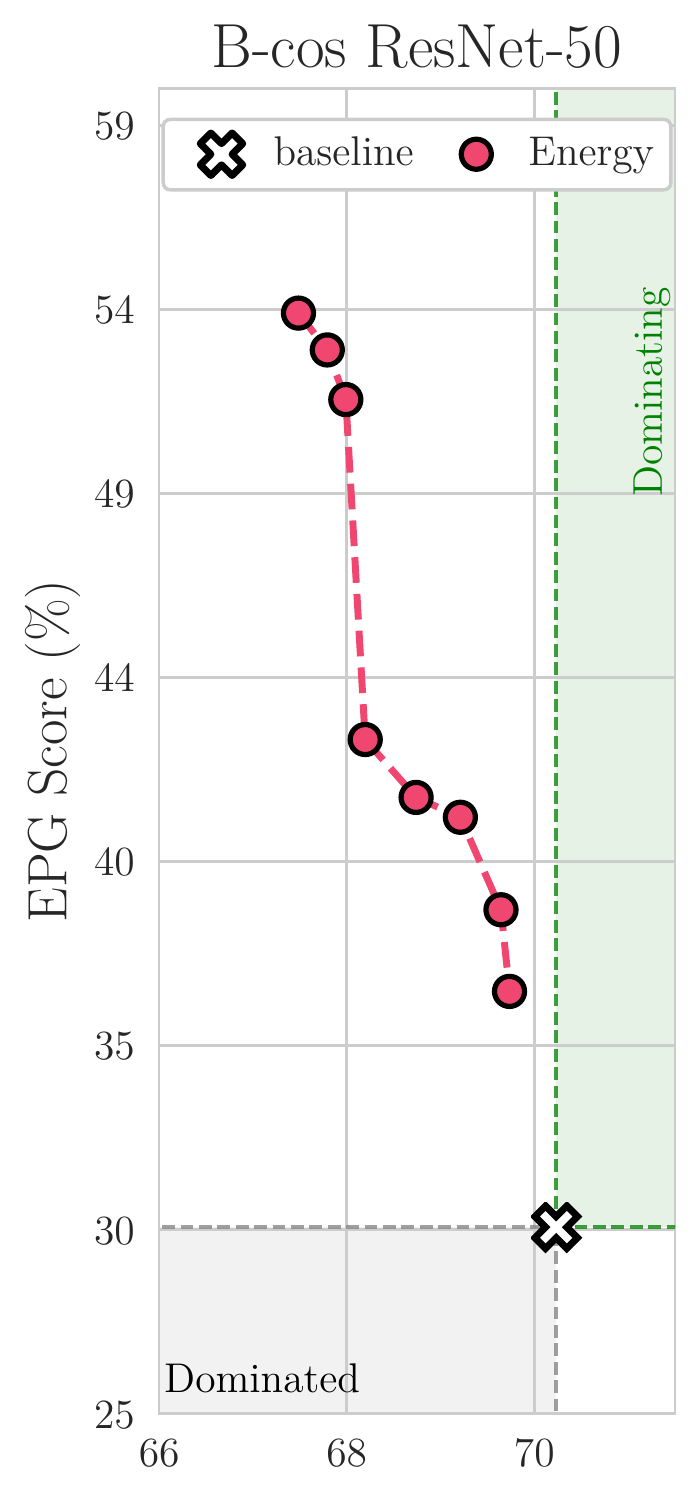}
    \caption{\textbf{The Pareto front.}}
    \label{fig:supp:pareto_front_quali:b}
    \end{subfigure}
    \caption{\textbf{Visualizing examples across the Pareto front.} We show \textbf{(a)} qualitative examples of attributions from models across the Pareto front for a single configuration (\bcos attributions, \energyloss localization loss, Input layer), and \textbf{(b)} the Pareto front curve. From left to right, attributions from each model on the curve (\textbf{(b)}) are visualized in column (\textbf{(a)}), in decreasing order of \epg scores. We find that models with better \epg scores also provide attributions that are better localized to bounding boxes for individual examples.}
    \label{fig:supp:pareto_front_quali}
\end{figure}
