# Supplementary material for: Studying How to Efficiently and Effectively Guide Models with Explanations
Source: arXiv:2303.11932 source file (2024-07-21)
Supplement: Supplementary file 2 [file quali_pareto_front.tex]

\begin{figure}[hb]
    \centering
    \textbf{Pareto-front visualization (\cocos).}\\\vspace{.25cm}
    \begin{subfigure}[c]{.76\textwidth}
    \includegraphics[width=\textwidth]{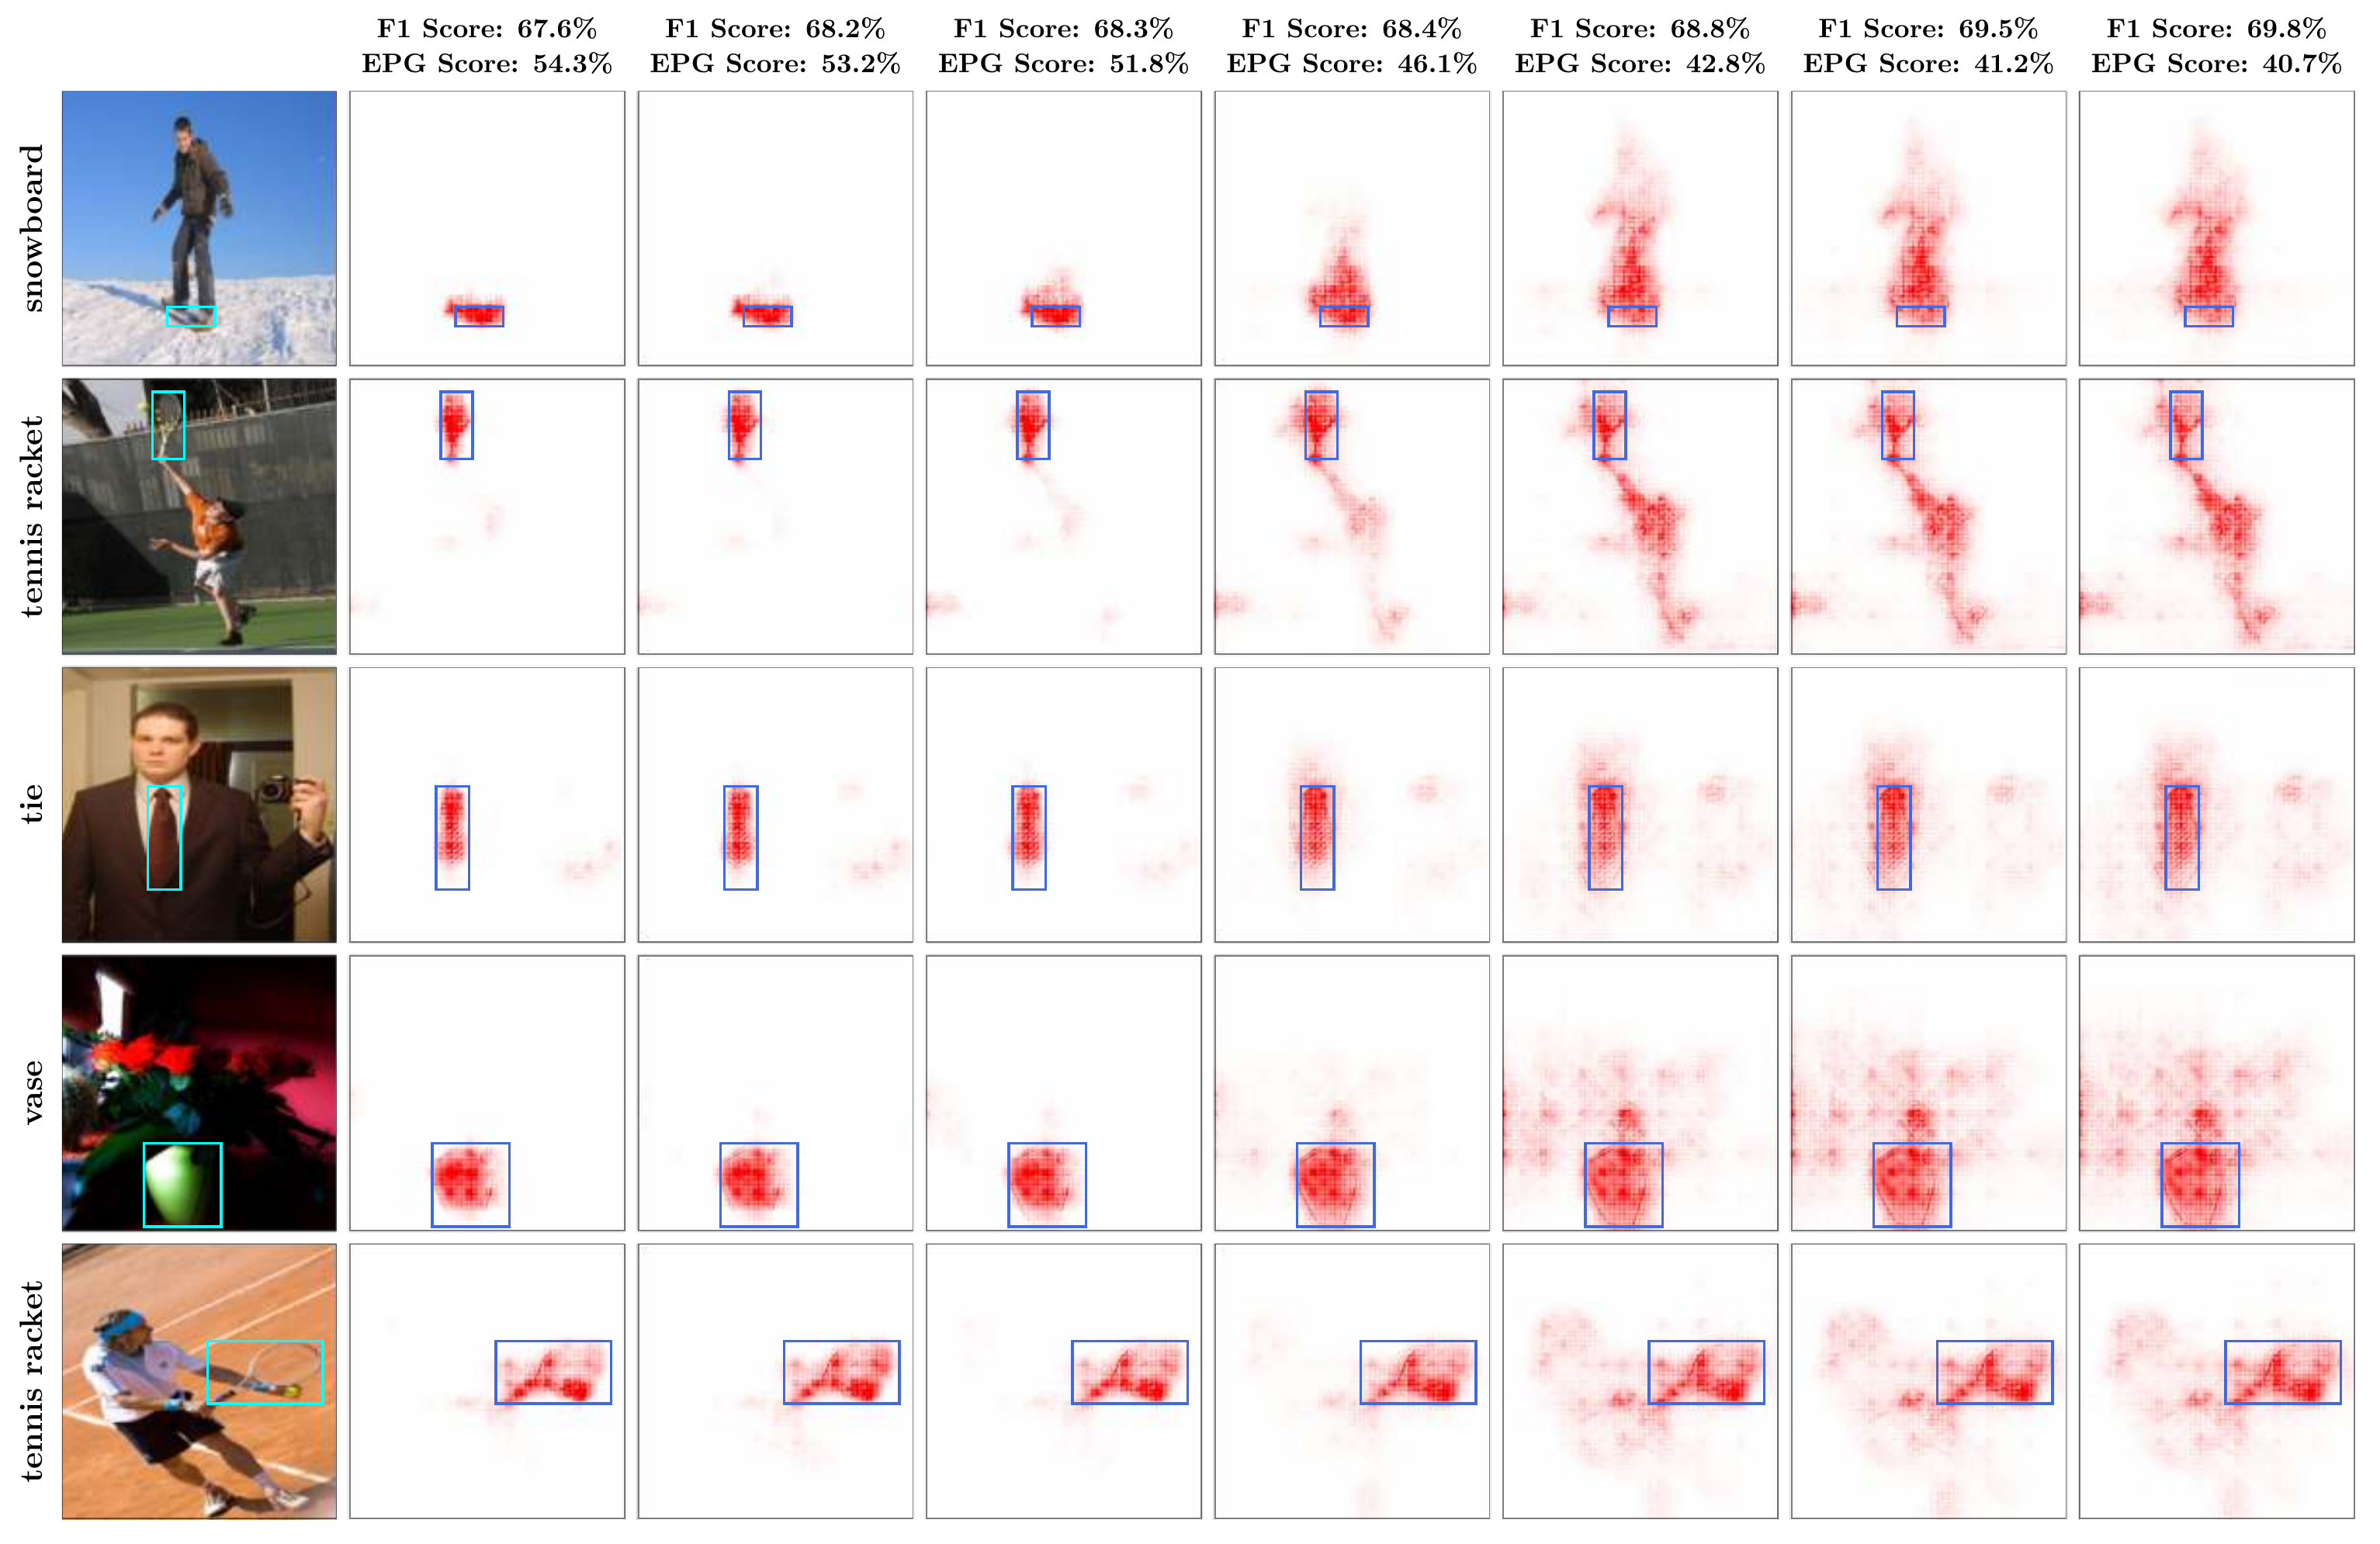}
    \caption{\textbf{Qualitative Examples from across the Pareto front.}}
    \label{fig:supp:pareto_front_quali:a}
    \end{subfigure}\hfill
    \begin{subfigure}[c]{.2275\textwidth}
    \includegraphics[width=\textwidth]{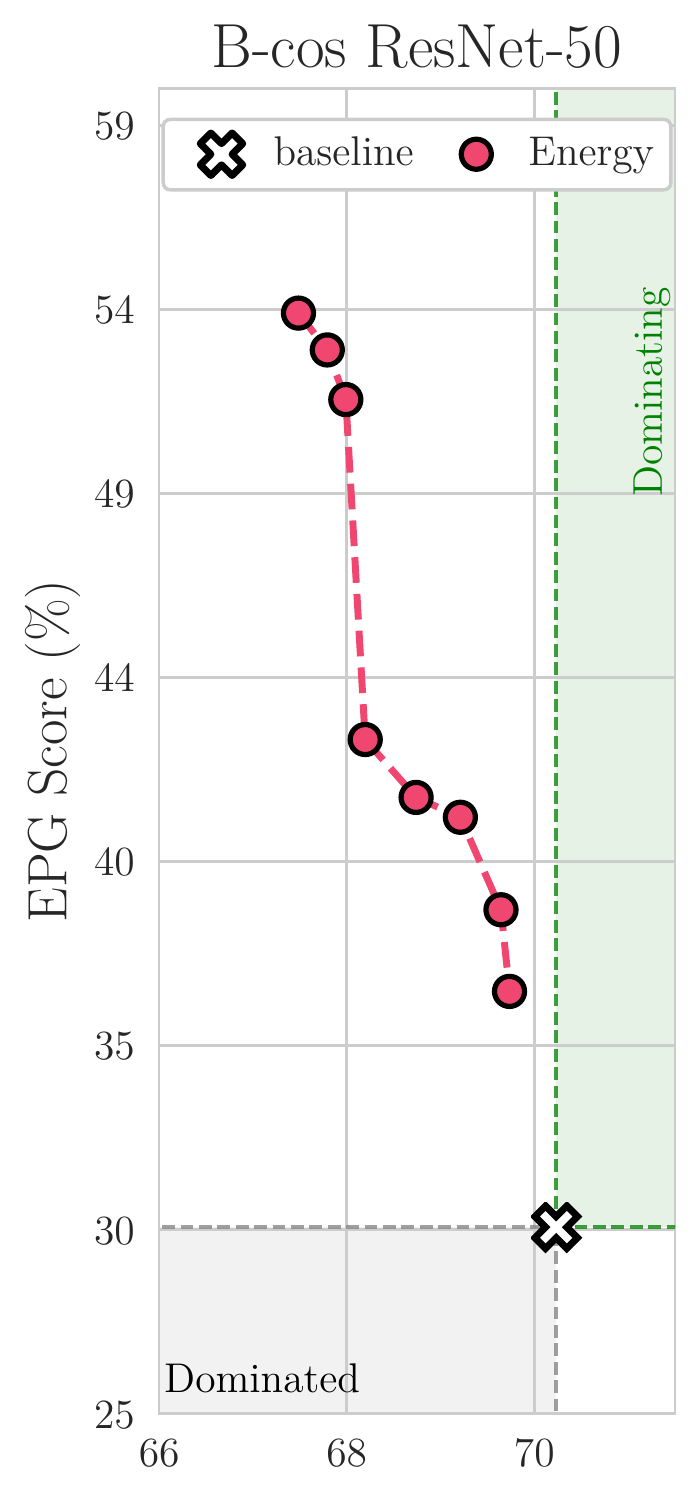}
    \caption{\textbf{The Pareto front.}}
    \label{fig:supp:pareto_front_quali:b}
    \end{subfigure}
    \caption{\textbf{Visualizing examples across the Pareto front.} We show \textbf{(a)} qualitative examples of attributions from models across the Pareto front for a single configuration (\bcos attributions, \energyloss localization loss, Input layer), and \textbf{(b)} the Pareto front curve. From left to right, attributions from each model on the curve (\textbf{(b)}) are visualized in column (\textbf{(a)}), in decreasing order of \epg scores. We find that models with better \epg scores also provide attributions that are better localized to bounding boxes for individual examples.}
    \label{fig:supp:pareto_front_quali}
\end{figure}
